# Supplementary material for: Giant Ferrimagnetism and Polarization in a Mixed Metal Perovskite Metal-Organic Framework
Source: arXiv:1703.10853 source file (2018-01-17)
Supplement: Supplementary file 1 [file SupplementaryInformation.pdf]

# Supplementary Information

## DETAILS OF DFT CALCULATIONS

### Code and parameters

The spin-polarized GGA calculations in this work employed the Quantum ESPRESSO code [1] and used the Perdew-Burke-Ernzerhof [2, 3] exchange-correlation functional. Ionic cores were modeled by PAW pseudopotentials [4, 5](for details see theossrv1.epfl.ch/Main/Pseudopotentials). We used a $7 \times 7 \times 5$ Monkhorst-Pack k-point mesh for Brillouin zone integration and a plane-wave basis with a 60 Ry kinetic-energy cutoff along with a 480 Ry cutoff for the charge-density. These values ensured good convergence in energies and forces. Structures were relaxed until the forces were less than 13 meV/Å. Volumes and lattice parameters of cells considered were optimized until the stresses were less than 0.5 Kbar.

Correlation effects due to the $3d$ transition metals in the system can be accounted for by using a Hubbard $U$ correction to the GGA functional [6–8]. The simplified version of GGA+$U$ functional given by Coccocioni *et al* [9, 10] and as implemented in Quantum-ESPRESSO was used. The Hubbard $U$ parameter can be calculated *ab initio* using the linear response formalism [9, 10] or a self consistent approach (SCF) [7, 8, 11]. Using the latter method we calculated the $U$ values to be 4.0 eV (Cu) and 3.5 eV (Mn) in $[C(NH_3)_2][Cu_{0.5}Mn_{0.5}(HCOO)_3]$. Ferroelectric polarization values were calculated using the Berry phase approach [12] based on the GGA+U+vdW functional.

We also included spin-orbit coupling (SOC) on both Cu and Mn atoms to check for any non-collinear magnetic ground states in the mixed metal MOF but did not observe any significant change in magnetization along the $z$-axis. Although the moments developed components in the $xy$-plane of small magnitudes, the electronic structure did not change significantly. Therefore, for most of the structural and energetic discussions we have excluded SOC effects. We confine the discussion of the results of the SOC calculations to the context of the magnetoelectric effect below.

As a validation of our method, we first used it to reproduce the previously calculated properties of parent Cu-MOF [13]. We found that the results on the electronic and magnetic properties, from the previous studies are in good agreement with our GGA+$U$+vdW calculations. The GGA+$U$ method has been successfully used in describing magnetic properties of inorganic transition metal oxides [14–17] and MOFs [18]. So, this is an attractive alternative to the more computationally expensive hybrid HSE06 [19] method often used in this context. We also calculated the polarization in the Cu-MOF using the Berry phase approach to be 0.36 $\mu$ C/cm$^2$ which agrees with the previously calculated value (0.37 $\mu$ C/cm$^2$) [13].

## MAGNETIC AND CATION ORDERING STRUCTURES

We have taken three possible types of AFM ordered structures - A, C, G-types and FM ordered structures as shown in Fig.1(a). In each of these magnetic orders we further allowed for various ordering of the TM cations by considering three different arrangements of Mn/Cu ions in the supercell, termed as D0, D1, D2 in the Fig. 1(b). All the structures were fully relaxed and the final GGA+U+vdW energies indicated (See main text Fig.2) that the structure D1-A emerged as ground state structure with lowest energy.

## STRUCTURAL OPTIMIZATION

$ABX_3$ MOFs have been synthesized in $Pnna$ and $Pna2_1$ space groups[20]. Mixing of metals at the B-site lowers the symmetry but for comparison we still refer to the space groups of the parent MOFs. For instance, the ground state polar structure of $[C(NH_3)_2][Cu_{0.5}Mn_{0.5}(HCOO)_3]$ was found to be $Pna2_1$-like with a slight monoclinic distortion. The non-polar reference phase, taken to be a *Pnna*-like centric structure, had an energy of 0.37 Ry/cell greater than the polar phase.

### Structural parameters of $[C(NH_3)_2][Cu_{0.5}Mn_{0.5}(HCOO)_3]$

Full structural optimization of the $Pna2_1$-like structure was performed using the GGA+$U$+vdW functional in all combination of cation and magnetic orderings. We summarize some important aspects of the ground-state structure (D1-A) in Table I. The atomic positions calculated from the GGA+U+vdW cell optimization follow.

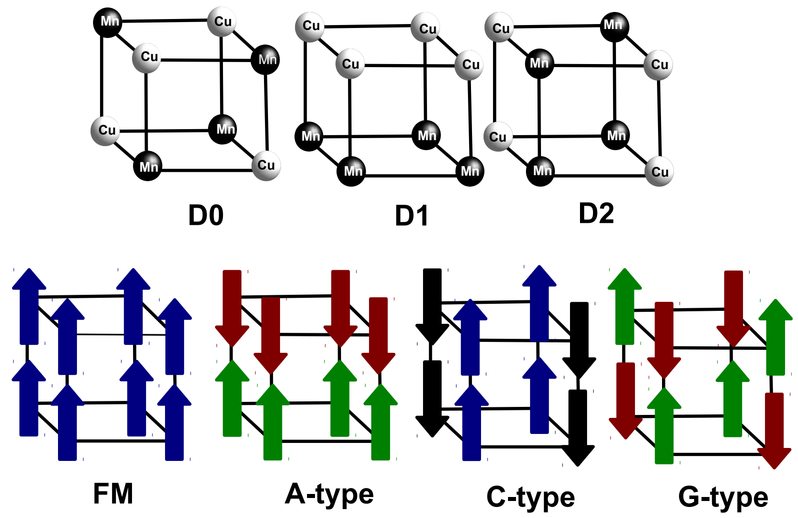


FIG. 1. Different types of cells considered in the calculations differing in : (a) Possible cation (Mn/Cu) ordering, which provides D0, D1 and D2 structures, and (b) magnetic ordering, where with up and down arrows representing up and down spins, respectively. FM refers to a ferromagnetic ordering where as A-, C- and G-types are different types of antiferromagnetic orderings.

TABLE I. Comparison of Cu-Mn bond distances (see Fig. S1) and major O-H bond length of ($Cu_{0.5}Mn_{0.5}$)-MOF for both polar ($\lambda = \pm 1$) and non-polar ($\lambda = 0$) D1-A structures. $\lambda = -1$ corresponds to the inverted polar structure.

| Length (Å) | $\lambda = -1$ | $\lambda = 0$ | $\lambda = +1$ |
|---|---|---|---|
| d(Mn1-Mn2) | 6.20 | 6.20 | 6.20 |
| d(Cu1-Cu2) | 6.25 | 6.20 | 6.16 |
| d(Cu1-Mn1) | 5.82 | 5.81 | 5.79 |
| d(Cu2-Mn2) | 5.82 | 5.81 | 5.79 |
| d(O-H(1)) | 1.83 | 1.90 | 1.96 |
| d(O-H(2)) | 1.92 | 1.90 | 1.84 |
| d(Cu-O)$_{eq1}$ | 2.02, 1.99 | 2.32, 2.27 | 2.44, 2.36 |
| d(Cu-O)$_{ax}$ | 2.02, 2.04 | 2.11, 2.11 | 2.04, 2.02 |
| d(Cu-O)$_{eq2}$ | 2.44, 2.36 | 2.26, 2.30 | 1.99, 2.02 |
| d(Mn-O)$_{eq1}$ | 2.17, 2.20 | 2.26, 2.30 | 2.17, 2.21 |
| d(Mn-O)$_{ax}$ | 2.22, 2.22 | 2.11, 2.11 | 2.22, 2.22 |
| d(Mn-O)$_{eq2}$ | 2.18, 2.21 | 2.32, 2.27 | 2.21, 2.17 |

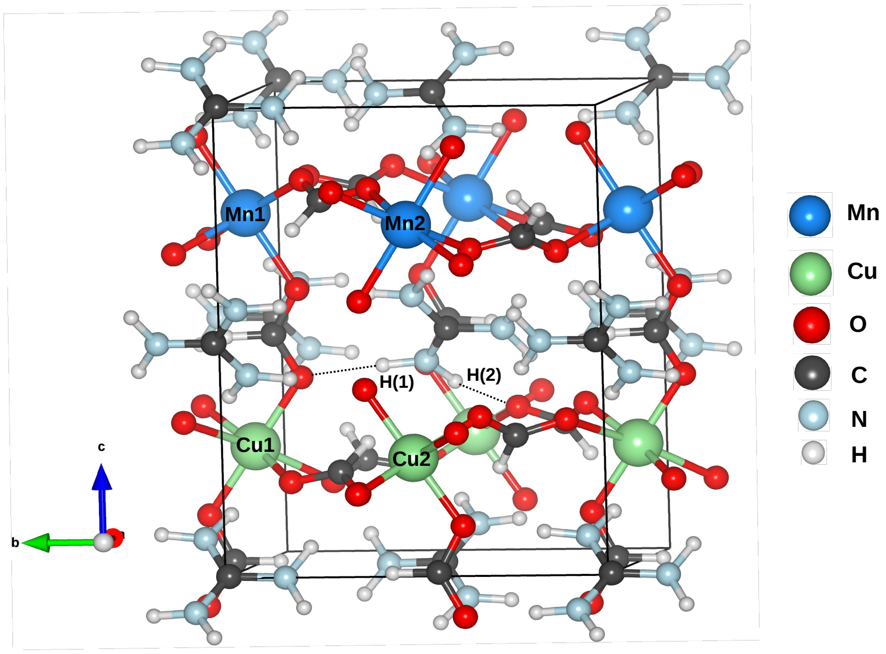


FIG. 2. Fully optimized crystal structure of polar ($Pna2_1$ ) with octahedral orientation.

**1. Optimized atomic positions for Pna$2_1$-like (Cu0.5Mn0.5)-MOF (D1-A) (λ =+1) from GGA+U+vdW calculations. Lattice constants : a= 8.44230 Å, b=9.09184 Å, c=11.59540 Å. $\alpha = \gamma = 90^\circ$ and $\beta = 91.16^\circ$ . Total Energy = -2676.44720520 Ry**

| | | | |
|---|---|---|---|
| Cu | 0.018362608 | 0.503193354 | 0.251521709 |
| Cu | 0.518362428 | 0.996806571 | 0.251521705 |
| Mn | 0.981288458 | 0.500064998 | 0.749990002 |
| Mn | 0.481288460 | -0.000065069 | 0.749990028 |
| O | 0.339195440 | 0.829010080 | 0.827801098 |
| O | 0.648252873 | 0.151835450 | 0.330196308 |
| O | 0.148253229 | 0.348164296 | 0.330196273 |
| O | 0.839196254 | 0.670989492 | 0.827801055 |
| O | 0.689580286 | 0.823598866 | 0.166150743 |
| O | 0.328774809 | 0.166076232 | 0.671858307 |
| O | 0.828775112 | 0.333924149 | 0.671858022 |
| O | 0.189579785 | 0.676400876 | 0.166150288 |
| O | 0.679524619 | 0.132604414 | 0.684715279 |
| O | 0.339542812 | 0.877024012 | 0.184314260 |
| O | 0.839542875 | 0.622975986 | 0.184314257 |
| O | 0.179524381 | 0.367395847 | 0.684715401 |
| O | 0.296314065 | 0.146590701 | 0.315052741 |
| O | 0.684599613 | 0.869202658 | 0.815384173 |
| O | 0.184599351 | 0.630796330 | 0.815384379 |
| O | 0.796313603 | 0.353407855 | 0.315052580 |
| O | 0.485030078 | 0.126203083 | 0.913860415 |
| O | 0.519800577 | 0.873823815 | 0.397201511 |
| O | 0.019801129 | 0.626176068 | 0.397201401 |
| O | 0.985029602 | 0.373797145 | 0.913860847 |
| O | 0.518306369 | 0.121598409 | 0.105380231 |
| O | 0.481010717 | 0.871653969 | 0.587040947 |
| O | 0.981011159 | 0.628346234 | 0.587040847 |
| O | 0.018305892 | 0.378401822 | 0.105380243 |
| N | 0.514899991 | 0.654779442 | 0.999333158 |
| N | 0.494127624 | 0.338929566 | 0.499716626 |
| N | 0.994127059 | 0.161070194 | 0.499717396 |
| N | 0.014899770 | 0.845219363 | 0.999332689 |
| N | 0.408718586 | 0.435587426 | 0.931731399 |
| N | 0.592191860 | 0.556739779 | 0.426597436 |
| N | 0.092191107 | 0.943260642 | 0.426597936 |
| N | 0.908718318 | 0.064411841 | 0.931731401 |
| N | 0.599725750 | 0.434011512 | 0.078446160 |
| N | 0.411718868 | 0.560643293 | 0.575479631 |

| | | | |
|---|---|---|---|
| N | 0.911717741 | 0.939356594 | 0.575480286 |
| N | 0.099725065 | 0.065988000 | 0.078445815 |
| C | 0.216836814 | 0.762471139 | 0.790508292 |
| C | 0.759841830 | 0.225948293 | 0.284346386 |
| C | 0.259841439 | 0.274053572 | 0.284345768 |
| C | 0.716835771 | 0.737530067 | 0.790508156 |
| C | 0.808683187 | 0.757980800 | 0.206463787 |
| C | 0.210970901 | 0.235501309 | 0.710250222 |
| C | 0.710970555 | 0.264498154 | 0.710250085 |
| C | 0.308683818 | 0.742019607 | 0.206463980 |
| C | 0.502144655 | 0.058078466 | 0.008337707 |
| C | 0.486615080 | 0.937471043 | 0.491230134 |
| C | 0.986615589 | 0.562528960 | 0.491229920 |
| C | 0.002144199 | 0.441920922 | 0.008337579 |
| C | 0.507661886 | 0.508392884 | 0.003286708 |
| C | 0.498973049 | 0.485449052 | 0.500238040 |
| C | 0.998974210 | 0.014551213 | 0.500237107 |
| C | 0.007661876 | 0.991608598 | 0.003286827 |
| H | 0.133702895 | 0.822846617 | 0.732104949 |
| H | 0.825862270 | 0.172396323 | 0.213916608 |
| H | 0.325862131 | 0.327603846 | 0.213916586 |
| H | 0.633702696 | 0.677153271 | 0.732104985 |
| H | 0.892660871 | 0.817230084 | 0.264612357 |
| H | 0.131257001 | 0.177342096 | 0.770188945 |
| H | 0.631257040 | 0.322657630 | 0.770188753 |
| H | 0.392660515 | 0.682769964 | 0.264612442 |
| H | 0.502963033 | 0.936974847 | 0.007281167 |
| H | 0.460441515 | 0.056181556 | 0.487928769 |
| H | 0.960441856 | 0.443818464 | 0.487928950 |
| H | 0.002962752 | 0.563025330 | 0.007280990 |
| H | 0.448504458 | 0.711284529 | 0.938772699 |
| H | 0.553586242 | 0.279571059 | 0.438790592 |
| H | 0.053586597 | 0.220429293 | 0.438790300 |
| H | 0.948504694 | 0.788715731 | 0.938772706 |
| H | 0.581983666 | 0.711955337 | 0.059866212 |
| H | 0.429357824 | 0.283831555 | 0.560071444 |
| H | 0.929358160 | 0.216168279 | 0.560071209 |
| H | 0.081983661 | 0.788044701 | 0.059866030 |
| H | 0.582074740 | 0.323423284 | 0.089104669 |
| H | 0.423999568 | 0.672710005 | 0.580490685 |
| H | 0.923999518 | 0.827289782 | 0.580490727 |
| H | 0.082074323 | 0.176576687 | 0.089104663 |

| | | | |
|---|---|---|---|
| H | 0.418707616 | 0.323435088 | 0.925473944 |
| H | 0.583120277 | 0.668557575 | 0.418237724 |
| H | 0.083120203 | 0.831442565 | 0.418237783 |
| H | 0.918707264 | 0.176565176 | 0.925473953 |
| H | 0.685177312 | 0.489472274 | 0.125205641 |
| H | 0.327610182 | 0.505126994 | 0.620828688 |
| H | 0.827610453 | 0.994872539 | 0.620828594 |
| H | 0.185177212 | 0.010527713 | 0.125205621 |
| H | 0.328252826 | 0.494515210 | 0.883015787 |
| H | 0.668046410 | 0.495351600 | 0.377676739 |
| H | 0.168046416 | 1.004648804 | 0.377676698 |
| H | 0.828252633 | 0.005484819 | 0.883015716 |

-----------------------------------------------------------------------------------------------------

**2. Optimized atomic positions for Pna$2_1$-like (Cu0.5Mn0.5)-MOF (D0-G) (λ = +1) from GGA+U+vdW calculations. Lattice constants : a= 8.43548 Å, b=9.08203 Å, c=11.60624 Å and $\alpha = 90.76°$, $\beta = 91.18°$ and $\gamma = 86.94°$. Total Energy = -2676.44582190 Ry**

| | | | |
|---|---|---|---|
| Cu | 0.018055283 | 0.497994238 | 0.247466313 |
| Mn | 0.518740586 | 0.997146256 | 0.253396550 |
| Mn | 0.981267466 | 0.502835809 | 0.746591376 |
| Cu | 0.481962690 | 0.001980691 | 0.752532695 |
| O | 0.322919806 | 0.828726145 | 0.834917049 |
| O | 0.665653648 | 0.159975643 | 0.331001103 |
| O | 0.151908864 | 0.337943500 | 0.325837711 |
| O | 0.827221738 | 0.674535113 | 0.825715355 |
| O | 0.672755290 | 0.825480750 | 0.174242121 |
| O | 0.348106915 | 0.161967400 | 0.674137422 |
| O | 0.834338625 | 0.340070314 | 0.668952984 |
| O | 0.177027282 | 0.671261472 | 0.165051490 |
| O | 0.701474638 | 0.135662276 | 0.689449357 |
| O | 0.321645605 | 0.869104032 | 0.189752640 |
| O | 0.834808152 | 0.624855449 | 0.179676914 |
| O | 0.183189049 | 0.360247388 | 0.682607434 |
| O | 0.316850636 | 0.139675766 | 0.317442664 |
| O | 0.665152857 | 0.875151950 | 0.820375976 |
| O | 0.178309444 | 0.630861373 | 0.810316460 |
| O | 0.798617315 | 0.364344002 | 0.310633002 |
| O | 0.477294025 | 0.124228906 | 0.899686971 |
| O | 0.521177952 | 0.872331965 | 0.416632021 |
| O | 0.017245868 | 0.621185924 | 0.393692837 |
| O | 0.990427810 | 0.374210969 | 0.908949608 |
| O | 0.509447089 | 0.125826533 | 0.091048707 |

| | | | |
|---|---|---|---|
| O | 0.482953052 | 0.878783075 | 0.606294530 |
| O | 0.979077039 | 0.627651020 | 0.583361452 |
| O | 0.022622823 | 0.375770961 | 0.100306861 |
| N | 0.508167602 | 0.655489343 | 0.998067217 |
| N | 0.492310343 | 0.340819057 | 0.499678994 |
| N | 1.007697441 | 0.159163841 | 0.500304420 |
| N | -0.008241927 | 0.844544952 | 1.001911990 |
| N | 0.409700572 | 0.439910152 | 0.925308772 |
| N | 0.583571403 | 0.557797116 | 0.431150795 |
| N | 0.094997575 | 0.935919066 | 0.418738728 |
| N | 0.898996986 | 0.069768070 | 0.928030096 |
| N | 0.600965892 | 0.430288206 | 0.071969558 |
| N | 0.404953558 | 0.564073083 | 0.581207688 |
| N | 0.916439958 | 0.942182996 | 0.568832884 |
| N | 0.090332151 | 0.060093521 | 0.074642767 |
| C | 0.206013509 | 0.765359154 | 0.792974004 |
| C | 0.777788158 | 0.230941790 | 0.289997339 |
| C | 0.270304735 | 0.265835471 | 0.282915973 |
| C | 0.701357176 | 0.742876446 | 0.790787108 |
| C | 0.798601270 | 0.757141878 | 0.209223315 |
| C | 0.229776108 | 0.234104074 | 0.717134352 |
| C | 0.722249293 | 0.269093714 | 0.710010323 |
| C | 0.293895111 | 0.734611566 | 0.207071230 |
| C | 0.488492854 | 0.059379881 | -0.003813906 |
| C | 0.516422422 | 0.939721576 | 0.512441203 |
| C | 0.983721530 | 0.560273083 | 0.487545117 |
| C | 0.011445473 | 0.440637250 | 0.003814271 |
| C | 0.506274988 | 0.508812100 | -0.001232419 |
| C | 0.493431653 | 0.487522936 | 0.503848919 |
| C | 1.006565710 | 0.012463166 | 0.496123431 |
| C | -0.006303899 | 0.991218144 | 0.001212115 |
| H | 0.120648884 | 0.829252927 | 0.736147473 |
| H | 0.861990269 | 0.169533853 | 0.231876921 |
| H | 0.333772439 | 0.316472205 | 0.212065025 |
| H | 0.619212130 | 0.686142602 | 0.731685785 |
| H | 0.880714486 | 0.813901439 | 0.268333936 |
| H | 0.166424744 | 0.183491071 | 0.788054991 |
| H | 0.638037278 | 0.330519270 | 0.768112318 |
| H | 0.379178220 | 0.670703755 | 0.263952416 |
| H | 0.478572036 | 0.938990313 | -0.003899386 |
| H | 0.543778364 | 0.057044590 | 0.516122301 |
| H | 0.956193329 | 0.442992784 | 0.483849724 |

| | | | |
|---|---|---|---|
| H | 0.021459880 | 0.561015325 | 0.003903901 |
| H | 0.438013805 | 0.714694058 | 0.939014590 |
| H | 0.555867458 | 0.282077378 | 0.437912127 |
| H | 0.067470044 | 0.215214453 | 0.440182525 |
| H | 0.928660778 | 0.789905769 | 0.939657838 |
| H | 0.571251346 | 0.710142624 | 0.060322231 |
| H | 0.432506468 | 0.284771009 | 0.559782125 |
| H | 0.944144511 | 0.217907077 | 0.562073087 |
| H | 0.061932868 | 0.785321551 | 0.060941526 |
| H | 0.585095131 | 0.319844178 | 0.080229384 |
| H | 0.412936207 | 0.675871794 | 0.588319734 |
| H | 0.929696169 | 0.829501038 | 0.574415364 |
| H | 0.077709891 | 0.172482629 | 0.083790832 |
| H | 0.422301706 | 0.327515646 | 0.916200643 |
| H | 0.570368684 | 0.670486047 | 0.425592350 |
| H | 0.087067784 | 0.824109129 | 0.411654963 |
| H | 0.914866776 | 0.180214440 | 0.919784068 |
| H | 0.683597044 | 0.482430963 | 0.120970897 |
| H | 0.322953329 | 0.510488216 | 0.626125286 |
| H | 0.838730309 | 1.004654071 | 0.619535226 |
| H | 0.173168152 | -0.002274652 | 0.121997064 |
| H | 0.326817905 | 0.502260445 | 0.877980171 |
| H | 0.661335360 | 0.495322925 | 0.380489402 |
| H | 0.177002228 | 0.989504554 | 0.373821172 |
| H | 0.816344805 | 0.017643965 | 0.879036090 |

---

**3. Optimized atomic positions for Pna2$_1$-like (Cu0.5Mn0.5)-MOF (D2-G) from GGA+U+vdW calculations. Lattice constants : a= 8.39858 Å, b=9.07849 Å, c=11.63825 Å and $\alpha = \gamma = 90^\circ$ and $\beta = 86.81^\circ$. Total Energy = -2676.4352478917 Ry**

| | | | |
|---|---|---|---|
| Cu | 0.014697194 | 0.497548753 | 0.249425239 |
| Mn | 0.519467280 | 0.997732690 | 0.253157464 |
| Cu | 0.985302573 | 0.502451292 | 0.749424330 |
| Mn | 0.480532615 | 0.002266928 | 0.753157673 |
| O | 0.332888009 | 0.842794321 | 0.832945175 |
| O | 0.667112156 | 0.157205375 | 0.332945022 |
| O | 0.145562288 | 0.336343696 | 0.324107876 |
| O | 0.854437873 | 0.663656668 | 0.824107621 |
| O | 0.681414986 | 0.831054881 | 0.172028058 |
| O | 0.318585995 | 0.168944225 | 0.672027584 |
| O | 0.824177959 | 0.326259850 | 0.669321627 |

| | | | |
|---|---|---|---|
| O | 0.175820419 | 0.673739778 | 0.169321832 |
| O | 0.679209819 | 0.128502817 | 0.689809646 |
| O | 0.320789294 | 0.871496935 | 0.189809941 |
| O | 0.838630910 | 0.627003334 | 0.182524724 |
| O | 0.161369230 | 0.372995635 | 0.682524100 |
| O | 0.313194664 | 0.139131036 | 0.318463918 |
| O | 0.686805322 | 0.860869941 | 0.818464293 |
| O | 0.199422160 | 0.638650374 | 0.808681624 |
| O | 0.800578568 | 0.361348638 | 0.308681871 |
| O | 0.475590813 | 0.137138345 | 0.908325334 |
| O | 0.524408613 | 0.862862149 | 0.408326063 |
| O | 0.007422472 | 0.616138071 | 0.402945885 |
| O | 0.992577377 | 0.383862370 | 0.902945390 |
| O | 0.516249497 | 0.134454808 | 0.098187071 |
| O | 0.483750838 | 0.865545426 | 0.598187500 |
| O | 0.975151538 | 0.618827669 | 0.593398005 |
| O | 0.024848625 | 0.381172044 | 0.093397664 |
| N | 0.517162760 | 0.664267622 | 0.998562480 |
| N | 0.482836604 | 0.335728504 | 0.498562624 |
| N | 0.998441951 | 0.152509951 | 0.501019916 |
| N | 0.001558154 | 0.847492174 | 1.001020103 |
| N | 0.415010391 | 0.449688598 | 0.930744725 |
| N | 0.584989342 | 0.550308690 | 0.430745254 |
| N | 0.092185298 | 0.928848810 | 0.423593738 |
| N | 0.907815021 | 0.071152729 | 0.923593248 |
| N | 0.603446955 | 0.438835984 | 0.076682909 |
| N | 0.396552658 | 0.561161352 | 0.576682948 |
| N | 0.910107013 | 0.934988294 | 0.574005689 |
| N | 0.089892516 | 0.065013397 | 0.074005671 |
| C | 0.220579770 | 0.772102699 | 0.789607625 |
| C | 0.779421270 | 0.227897911 | 0.289607733 |
| C | 0.267756925 | 0.265507107 | 0.283093436 |
| C | 0.732243643 | 0.734492464 | 0.783093319 |
| C | 0.801746000 | 0.759279313 | 0.212042566 |
| C | 0.198252461 | 0.240721334 | 0.712042343 |
| C | 0.706576813 | 0.263142411 | 0.708657322 |
| C | 0.293422937 | 0.736858146 | 0.208658051 |
| C | 0.484889709 | 0.072047173 | 0.004358580 |
| C | 0.515109820 | 0.927952161 | 0.504358369 |
| C | 0.982062491 | 0.551970554 | 0.497636706 |
| C | 0.017937685 | 0.448029771 | -0.002364141 |
| C | 0.512046024 | 0.517698339 | 0.002031812 |

| | | | |
|---|---|---|---|
| C | 0.487955375 | 0.482307179 | 0.502030977 |
| C | 1.000349774 | 0.005665205 | 0.499468626 |
| C | -0.000349558 | 0.994331701 | -0.000531357 |
| H | 0.136207333 | 0.833475484 | 0.730761396 |
| H | 0.863793910 | 0.166524366 | 0.230761502 |
| H | 0.334937518 | 0.317650119 | 0.213536379 |
| H | 0.665062918 | 0.682350408 | 0.713536590 |
| H | 0.878647875 | 0.812062795 | 0.275382926 |
| H | 0.121351282 | 0.187936811 | 0.775382225 |
| H | 0.620510981 | 0.327321091 | 0.764386069 |
| H | 0.379487221 | 0.672679060 | 0.264386820 |
| H | 0.463079861 | 0.953082195 | 0.006581992 |
| H | 0.536919101 | 0.046918219 | 0.506582019 |
| H | 0.964350847 | 0.432892942 | 0.496374881 |
| H | 0.035649833 | 0.567107005 | -0.003625618 |
| H | 0.450517571 | 0.723817401 | 0.938558479 |
| H | 0.549482618 | 0.276183014 | 0.438558148 |
| H | 0.058217262 | 0.208505027 | 0.439589487 |
| H | 0.941782594 | 0.791494687 | 0.939589240 |
| H | 0.581794958 | 0.718654623 | 0.058396661 |
| H | 0.418205654 | 0.281345949 | 0.558395855 |
| H | 0.932296362 | 0.211085594 | 0.562435807 |
| H | 0.067703177 | 0.788914208 | 0.062435901 |
| H | 0.588009061 | 0.328111151 | 0.085130229 |
| H | 0.411991562 | 0.671889654 | 0.585130438 |
| H | 0.924251752 | 0.822299835 | 0.580991947 |
| H | 0.075748295 | 0.177699492 | 0.080991672 |
| H | 0.427034504 | 0.337019123 | 0.922884610 |
| H | 0.572965631 | 0.662982149 | 0.422884461 |
| H | 0.083226681 | 0.817156702 | 0.416938798 |
| H | 0.916773666 | 0.182842859 | 0.916938712 |
| H | 0.687552772 | 0.489656877 | 0.123433214 |
| H | 0.312447779 | 0.510343459 | 0.623433088 |
| H | 0.828346212 | 0.996416214 | 0.622705533 |
| H | 0.171653495 | 0.003583299 | 0.122705627 |
| H | 0.336466441 | 0.513451377 | 0.880770571 |
| H | 0.663533977 | 0.486549253 | 0.380770310 |
| H | 0.173174773 | 0.982892973 | 0.376315123 |
| H | 0.826825639 | 0.017106961 | 0.876315113 |

**4. Optimized atomic positions for $Pna2_1$ -like (Cu0.5Mn0.5)-MOF (D1-A) (λ = -1) structure from GGA+U+vdW calculations. Lattice constants : a= 8.44166 Å, b=9.0922 Å, c=11.595 Å. $\alpha = \gamma = 90^\circ$ and $\beta = 88.9^\circ$ . Total Energy = -2676.4472052 Ry**

| | | | |
|---|---|---|---|
| Cu1 | 0.018308 | 0.496801 | 0.248510 |
| Cu2 | 0.518308 | 1.003200 | 0.248510 |
| Mn3 | 0.981298 | 0.499914 | 0.750012 |
| Mn4 | 0.481297 | 1.000086 | 0.750012 |
| O | 0.328952 | 0.833838 | 0.828111 |
| O | 0.689514 | 0.176402 | 0.333880 |
| O | 0.189516 | 0.323598 | 0.333881 |
| O | 0.828952 | 0.666163 | 0.828111 |
| O | 0.648284 | 0.848241 | 0.169863 |
| O | 0.339059 | 0.170910 | 0.672146 |
| O | 0.839060 | 0.329090 | 0.672147 |
| O | 0.148284 | 0.651760 | 0.169864 |
| O | 0.684495 | 0.130863 | 0.684570 |
| O | 0.296347 | 0.853327 | 0.185029 |
| O | 0.796346 | 0.646674 | 0.185029 |
| O | 0.184495 | 0.369137 | 0.684571 |
| O | 0.339451 | 0.122974 | 0.315663 |
| O | 0.679701 | 0.867481 | 0.815216 |
| O | 0.179701 | 0.632520 | 0.815216 |
| O | 0.839450 | 0.377026 | 0.315662 |
| O | 0.480993 | 0.128310 | 0.912964 |
| O | 0.518254 | 0.878359 | 0.394640 |
| O | 0.018253 | 0.621641 | 0.394640 |
| O | 0.980994 | 0.371689 | 0.912964 |
| O | 0.519768 | 0.126177 | 0.102819 |
| O | 0.484959 | 0.873759 | 0.586153 |
| O | 0.984961 | 0.626241 | 0.586154 |
| O | 0.019767 | 0.373824 | 0.102820 |
| N | 0.494376 | 0.661078 | 1.000251 |
| N | 0.514752 | 0.345190 | 0.500642 |
| N | 1.014751 | 0.154810 | 0.500643 |
| N | -0.005625 | 0.838922 | 1.000250 |
| N | 0.412046 | 0.439392 | 0.924382 |
| N | 0.599680 | 0.565943 | 0.421604 |
| N | 0.099679 | 0.934057 | 0.421605 |
| N | 0.912043 | 0.060608 | 0.924381 |
| N | 0.592353 | 0.443246 | 0.073436 |
| N | 0.408658 | 0.564392 | 0.568260 |

| | | | |
|---|---|---|---|
| N | 0.908657 | 0.935608 | 0.568260 |
| N | 0.092351 | 0.056754 | 0.073434 |
| C | 0.211131 | 0.764407 | 0.789695 |
| C | 0.808603 | 0.242011 | 0.293558 |
| C | 0.308602 | 0.257990 | 0.293560 |
| C | 0.711131 | 0.735592 | 0.789694 |
| C | 0.759845 | 0.774105 | 0.215768 |
| C | 0.216688 | 0.237438 | 0.709400 |
| C | 0.716687 | 0.262562 | 0.709400 |
| C | 0.259846 | 0.725896 | 0.215768 |
| C | 0.486367 | 0.062552 | 0.008811 |
| C | 0.502127 | 0.941870 | 0.491684 |
| C | 1.002128 | 0.558129 | 0.491684 |
| C | -0.013633 | 0.437449 | 0.008812 |
| C | 0.499212 | 0.514566 | -0.000279 |
| C | 0.507574 | 0.491575 | 0.496722 |
| C | 1.007575 | 0.008423 | 0.496721 |
| C | -0.000785 | 0.985434 | -0.000276 |
| H | 0.131396 | 0.822565 | 0.729741 |
| H | 0.892574 | 0.182738 | 0.235442 |
| H | 0.392574 | 0.317263 | 0.235442 |
| H | 0.631396 | 0.677435 | 0.729741 |
| H | 0.825812 | 0.827599 | 0.286275 |
| H | 0.133498 | 0.177027 | 0.767715 |
| H | 0.633497 | 0.322972 | 0.767715 |
| H | 0.325813 | 0.672402 | 0.286274 |
| H | 0.459760 | 0.943926 | 0.012173 |
| H | 0.503038 | 0.062970 | 0.492745 |
| H | 1.003039 | 0.437030 | 0.492745 |
| H | -0.040240 | 0.556074 | 0.012174 |
| H | 0.429636 | 0.716176 | 0.939852 |
| H | 0.581859 | 0.288020 | 0.440140 |
| H | 0.081859 | 0.211980 | 0.440140 |
| H | 0.929636 | 0.783824 | 0.939853 |
| H | 0.553783 | 0.720438 | 0.061224 |
| H | 0.448328 | 0.288682 | 0.561165 |
| H | 0.948328 | 0.211317 | 0.561164 |
| H | 0.053784 | 0.779561 | 0.061224 |
| H | 0.583246 | 0.331436 | 0.081784 |
| H | 0.418683 | 0.676539 | 0.574534 |
| H | 0.918683 | 0.823460 | 0.574534 |
| H | 0.083247 | 0.168564 | 0.081784 |

| | | | |
|---|---|---|---|
| H | 0.424223 | 0.327318 | 0.919443 |
| H | 0.582060 | 0.676530 | 0.410943 |
| H | 0.082060 | 0.823470 | 0.410943 |
| H | 0.924222 | 0.172682 | 0.919444 |
| H | 0.668143 | 0.504617 | 0.122445 |
| H | 0.328190 | 0.505492 | 0.616968 |
| H | 0.828191 | 0.994507 | 0.616968 |
| H | 0.168144 | -0.004617 | 0.122445 |
| H | 0.327875 | 0.494899 | 0.879048 |
| H | 0.685101 | 0.510468 | 0.374848 |
| H | 0.185102 | 0.989531 | 0.374848 |
| H | 0.827875 | 0.005100 | 0.879049 |

**5. Optimized atomic positions for $Pna2_1$-like (Cu0.5Mn0.5)-MOF (D0-G) (λ = -1) from GGA+U+vdW calculations. Lattice constants : a= 8.43682 Å, b=9.08203 Å, c=11.60454 Å and $\alpha = 90.77°$, $\beta = 88.82°$ and $\gamma = 93.12°$. Total Energy = -2676.44582190 Ry**

| | | | |
|---|---|---|---|
| Cu1 | 0.018152861 | 0.501956604 | 0.252458023 |
| Mn2 | 0.518851789 | 1.002770979 | 0.246660558 |
| Mn3 | 0.981154161 | 0.496901087 | 0.753341974 |
| Cu4 | 0.481822078 | -0.002255812 | 0.747534908 |
| O | 0.348134804 | 0.837662245 | 0.826065418 |
| O | 0.672827854 | 0.174469737 | 0.325994841 |
| O | 0.177105083 | 0.328527762 | 0.334622580 |
| O | 0.834267446 | 0.659730452 | 0.830816988 |
| O | 0.665728721 | 0.839933222 | 0.169181027 |
| O | 0.322896166 | 0.171143941 | 0.665376531 |
| O | 0.827187131 | 0.325195026 | 0.674004535 |
| O | 0.151852932 | 0.662025144 | 0.173934389 |
| O | 0.665002629 | 0.124554051 | 0.679471789 |
| O | 0.316892786 | 0.860325931 | 0.182337087 |
| O | 0.798634950 | 0.635642159 | 0.189584065 |
| O | 0.178211120 | 0.368862171 | 0.689877048 |
| O | 0.321790402 | 0.130807972 | 0.310122439 |
| O | 0.701361615 | 0.864022135 | 0.810410015 |
| O | 0.183111865 | 0.639348534 | 0.817664274 |
| O | 0.834996199 | 0.375121063 | 0.320526562 |
| O | 0.483112361 | 0.120977924 | 0.893753395 |
| O | 0.509165587 | 0.874037825 | 0.408984204 |
| O | 0.023044942 | 0.624155455 | 0.399637690 |
| O | 0.978359545 | 0.372131628 | 0.916600298 |
| O | 0.521647216 | 0.127529463 | 0.083398300 |
| O | 0.476944054 | 0.875523812 | 0.600364179 |

| | | | |
|---|---|---|---|
| O | 0.990836496 | 0.625628133 | 0.591017664 |
| O | 0.016882910 | 0.378698279 | 0.106247653 |
| N | 0.492514625 | 0.658992681 | 1.000402733 |
| N | 0.508170010 | 0.344372192 | 0.502125679 |
| N | 0.991837986 | 0.155294356 | 0.497874803 |
| N | 1.007477836 | 0.840664580 | 0.999598201 |
| N | 0.405151415 | 0.435697145 | 0.918827976 |
| N | 0.601026889 | 0.569633800 | 0.428262820 |
| N | 0.090458738 | 0.939778544 | 0.425215493 |
| N | 0.916153888 | 0.057582230 | 0.931159959 |
| N | 0.583843434 | 0.442076182 | 0.068839696 |
| N | 0.409548583 | 0.559887909 | 0.574784688 |
| N | 0.898980677 | 0.930032957 | 0.571737901 |
| N | 0.094838259 | 0.063958164 | 0.081177801 |
| C | 0.229608110 | 0.765583650 | 0.783232084 |
| C | 0.798602320 | 0.242876266 | 0.290885738 |
| C | 0.294102264 | 0.265284205 | 0.292783086 |
| C | 0.722214490 | 0.730644878 | 0.789743382 |
| C | 0.777784609 | 0.769021295 | 0.210250177 |
| C | 0.205898669 | 0.234387252 | 0.707218078 |
| C | 0.701412320 | 0.256793680 | 0.709118702 |
| C | 0.270388808 | 0.734092173 | 0.216766878 |
| C | 0.516739936 | 0.060096761 | 0.987589200 |
| C | 0.487580867 | 0.940365326 | 0.503833931 |
| C | 1.012411083 | 0.559305904 | 0.496165256 |
| C | -0.016742281 | 0.439569544 | 0.012408119 |
| C | 0.493656499 | 0.512291221 | 0.996188511 |
| C | 0.506259961 | 0.491037256 | 0.501409160 |
| C | 0.993747599 | 0.008629302 | 0.498590998 |
| C | 1.006336672 | 0.987366077 | 0.003813240 |
| H | 0.165984473 | 0.816333907 | 0.712535764 |
| H | 0.880481450 | 0.186207382 | 0.231559955 |
| H | 0.379563996 | 0.329272169 | 0.236058189 |
| H | 0.638113821 | 0.669202390 | 0.731532825 |
| H | 0.861891686 | 0.830463619 | 0.268455928 |
| H | 0.120440435 | 0.170398891 | 0.763944848 |
| H | 0.619547617 | 0.313462096 | 0.768455544 |
| H | 0.334011062 | 0.683331774 | 0.287458713 |
| H | 0.544093012 | 0.942793034 | 0.983881313 |
| H | 0.476485268 | 0.060603789 | 0.503880834 |
| H | 1.023499393 | 0.439066228 | 0.496111388 |
| H | -0.044102635 | 0.556871622 | 0.016109421 |

| | | | |
|---|---|---|---|
| H | 0.432693870 | 0.715004356 | 0.940315862 |
| H | 0.571419269 | 0.289724149 | 0.439964284 |
| H | 0.061923258 | 0.214511741 | 0.438766892 |
| H | 0.943900462 | 0.781888619 | 0.937828683 |
| H | 0.556095047 | 0.717769131 | 0.062170262 |
| H | 0.438084570 | 0.285154971 | 0.561233220 |
| H | 0.928588902 | 0.209942484 | 0.560036487 |
| H | 0.067295974 | 0.784651521 | 0.059686476 |
| H | 0.570663443 | 0.329376496 | 0.074382266 |
| H | 0.422215255 | 0.672280243 | 0.583958994 |
| H | 0.914875920 | 0.819613722 | 0.580020066 |
| H | 0.086890277 | 0.175754107 | 0.088297202 |
| H | 0.413106337 | 0.323901720 | 0.911707847 |
| H | 0.585133323 | 0.680052627 | 0.419981161 |
| H | 0.077788888 | 0.827386314 | 0.416040121 |
| H | 0.929335318 | 0.170281985 | 0.925618344 |
| H | 0.661530617 | 0.504607799 | 0.119561589 |
| H | 0.326744072 | 0.497485066 | 0.622175164 |
| H | 0.816252453 | 0.982091635 | 0.620677996 |
| H | 0.176890642 | 1.010429935 | 0.126036716 |
| H | 0.323101944 | 0.489225909 | 0.873967126 |
| H | 0.683754466 | 0.517572873 | 0.379322308 |
| H | 0.173261803 | 1.002181700 | 0.377823763 |
| H | 0.838465344 | -0.004946453 | 0.880436717 |

TABLE II. The optimized monoclinic structural parameters of the two different polar phase of D1 structure at $\lambda = \pm 1$ distortion. The total energies were given with respect to $\lambda = 0$ structure (monoclinic). The optimized orthorhombic lattice parameters are given in the bottom panel of the table.

| Distortion ($\lambda$) | Energy meV/TM | a (Å) | b (Å) | c (Å) | $\alpha$ (°) | $\beta$ (°) | $\gamma$ (°) |
|---|---|---|---|---|---|---|---|
| +1 | -1.8753 | 8.44 | 9.09 | 11.60 | 90.0 | 91.2 | 90.0 |
| -1 | -1.8732 | 8.44 | 9.09 | 11.60 | 90.0 | 88.9 | 90.0 |
| 0 | -0.6553 | 8.31 | 9.52 | 11.40 | 90.0 | 90.0 | 90.0 |

TABLE III. Formation energies for lowest energy magnetic structure of D0, D1 and D2 cation ordered structures.

| Structure Type | Energy of Formation ($\Delta E_f$) (meV/cell) |
|---|---|
| D0-G | -385 |
| D1-A | -404 |
| D2-G | -241 |

## FORMATION ENERGY

Starting from the experimental structure of Mn-MOF ([C($NH_2$)$_3$][Mn($HCOO$)$_3$]) (Pnna), we have computed the ground state of Mn-MOF to be G-type AFM. To the best of our knowledge, the ground magnetic state of the MOF has not been reported earlier. We used the predicted ground state of Mn-MOF for the calculation of formation energy. The enthalpy of formation is given by the equation below

$$\boxed{Cu - MOF(Pna2_1) + Mn - MOF(Pnna) \longrightarrow 2(Cu_{0.5}Mn_{0.5}) - MOF(Pna2_1)} \quad (1)$$

We optimized the structures of both the parent compounds Cu-MOF and Mn-MOF by using GGA+U+vdW functional, fixing the lattice parameters to the experimental values [20]. The optimized energies were then used in the above equation 1 to compute the enthalpy of formation for D0-A, D1-G and D2-G type structures. The calculated formation energies are given in the Table III. While all three structure seem stable compared to their parents we only considered the two most thermodynamically favorable structures, D1-A and D0-G, for our analysis.

## COUPLING CONSTANTS AND MONTE CARLO SIMULATIONS

In order to model the magnetic interactions we consider a rock-salt like unit cell formed by the TM sub-lattices as shown in Fig. 3. We consider the cell to be made up of two atomic layers (I and II) perpendicular to the $c$-axis. Each layer has 2 sites, $\alpha$ and $\beta$. Let $\vec{S}^{I,\alpha}_{i,j,k}$ refer to the spin of the atom in $(i,j,k)^{th}$ unit cell sitting in layer-I at site $\alpha$, and $\vec{S}^{I,\beta}_{i,j,k}$ to the spin of the atom at site $\beta$.

The following Heisenberg Hamiltonian describes the spin-spin interactions in the lattice of D0 structure

$$\begin{aligned} H = J_{\parallel} \sum_{i,j,k} \big[ & \vec{S}^{I,\alpha}_{i,j,k} \cdot \{ \vec{S}^{I,\beta}_{i,j,k} + \vec{S}^{I,\beta}_{i-1,j,k} + \vec{S}^{I,\beta}_{i,j-1,k} + \vec{S}^{I,\beta}_{i-1,j-1,k} \} \\ & + \vec{S}^{II,\alpha}_{i,j,k} \cdot \{ \vec{S}^{II,\beta}_{i,j,k} + \vec{S}^{II,\beta}_{i-1,j,k} + \vec{S}^{II,\beta}_{i,j-1,k} + \vec{S}^{II,\beta}_{i-1,j-1,k} \} \big] \\ & + J_{\perp} \sum_{i,j,k} \big[ \vec{S}^{I,\alpha}_{i,j,k} \cdot \{ \vec{S}^{II,\alpha}_{i,j,k-1} + \vec{S}^{II,\alpha}_{i,j,k+1} \} \\ & + \vec{S}^{I,\beta}_{i,j,k} \cdot \{ \vec{S}^{II,\beta}_{i,j,k-1} + \vec{S}^{II,\beta}_{i,j,k+1} \} \big] \end{aligned} \quad (2)$$

where $J_{\parallel}$ and $J_{\perp}$ are the in-plane and out-of-plane coupling constants, respectively; $i, j, k$ are site indices and $\vec{S}$ are spin vectors. Here, we treat the classical version of this Hamiltonian choosing the spin vectors to be parallel to the $z$-axis. Using Eq. 2 for different magnetically ordered supercells it is straightforward to extract the values of $J_{\parallel}$ and $J_{\perp}$ in terms of the corresponding supercell total energies and we obtain

$$\boxed{J_{\perp} = \frac{E_F + E_C - E_G - E_A}{20}, \; J_{\parallel} = \frac{E_F + E_A - E_G - E_C}{40}} \quad (3)$$

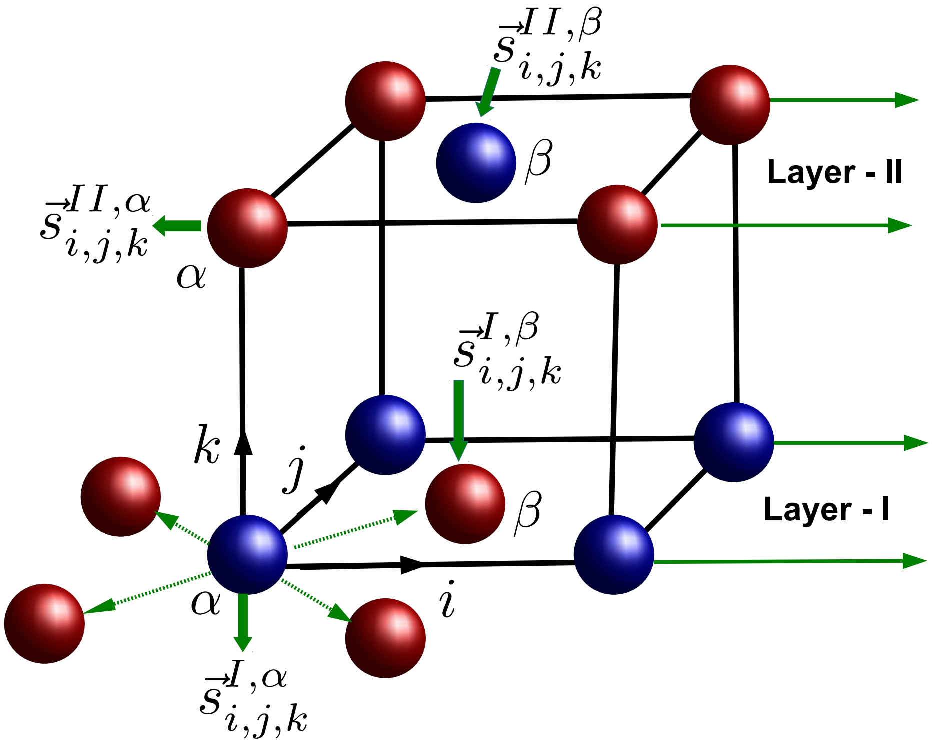


FIG. 3. Rock-salt like unit cell for the 3D Heisenberg model.

where $E_\kappa$ is the DFT energy of a unit cell with $\kappa$-type magnetic ordering. For D1, as there are two different in-plane superexchange ion pairs (Cu-Cu, Mn-Mn), there will be two separate coupling constants for each pair. The coupling constants can be calculated assuming the following Hamiltonian :

$$\begin{aligned} H = \sum_{i,j,k} J^I_\parallel [\vec{S}^{I,\alpha}_{i,j,k} \cdot \{\vec{S}^{I,\beta}_{i,j,k} + \vec{S}^{I,\beta}_{i-1,j,k} + \vec{S}^{I,\beta}_{i,j-1,k} + \vec{S}^{I,\beta}_{i-1,j-1,k}\}] \\ + J^{II}_\parallel [\vec{S}^{II,\alpha}_{i,j,k} \cdot \{\vec{S}^{II,\beta}_{i,j,k} + \vec{S}^{II,\beta}_{i-1,j,k} + \vec{S}^{II,\beta}_{i,j-1,k} + \vec{S}^{II,\beta}_{i-1,j-1,k}\}] \\ + J_\perp \sum_{i,j,k} [\vec{S}^{I,\alpha}_{i,j,k} \cdot \{\vec{S}^{II,\alpha}_{i,j,k-1} + \vec{S}^{II,\alpha}_{i,j,k+1}\} \\ + \vec{S}^{I,\beta}_{i,j,k} \cdot \{\vec{S}^{II,\beta}_{i,j,k-1} + \vec{S}^{II,\beta}_{i,j,k+1}\}] \end{aligned} \tag{4}$$

where, the superscript I and II refer to Mn and Cu, respectively. Using Eq. 4 we get,

$$\boxed{E_A = E_0 + J^{Cu}_\parallel + 25 \times J^{Mn}_\parallel - 5 \times J_\perp} \tag{5}$$

$$\boxed{E_C = E_0 - J^{Cu}_\parallel - 25 \times J^{Mn}_\parallel + 5 \times J_\perp} \tag{6}$$

$$\boxed{E_G = E_0 - J^{Cu}_\parallel - 25 \times J^{Mn}_\parallel - 5 \times J_\perp} \tag{7}$$

$$\boxed{E_F = E_0 + J^{Cu}_\parallel + 25 \times J^{Mn}_\parallel + 5 \times J_\perp} \tag{8}$$

where $E_0$ is the lattice contribution. Now, let us define

$$\boxed{E_Y = E_F - 5 \times J_\perp} \tag{9}$$

Hence, $E_Y$ will become

$$\boxed{E_Y = E_0 + J_{\parallel}^{Cu} + 25 \times J_{\parallel}^{Mn}} \tag{10}$$

Considering a spin configuration as provided in Fig.4 below and using Eq. 2 one would get

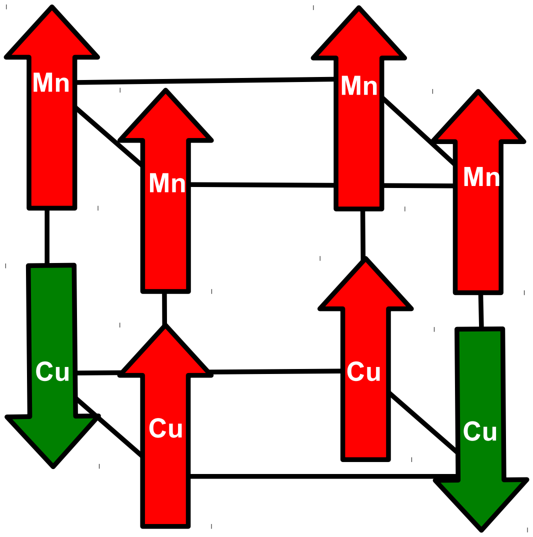


FIG. 4. Spin ordering to get the energy $E_X$ for D1-MOF .

$$\boxed{E_X = E_0 - J_{\parallel}^{Cu} + 25 \times J_{\parallel}^{Mn}} \tag{11}$$

Now, subtracting Eq. 11 from Eq. 10

$$\boxed{J_{\parallel}^{Cu} = \frac{E_Y - E_X}{2}} \tag{12}$$

Similarly defining,

$$\boxed{E_Z = E_C - 5 \times J_{\perp}} \implies \boxed{E_Z = E_0 - J_{\parallel}^{Cu} - 25 \times J_{\parallel}^{Mn}} \tag{13}$$

Now, again subtracting Eq. 13 from Eq. 11

$$\boxed{J_{\parallel}^{Mn} = \frac{E_X - E_Z}{50}} \tag{14}$$

A similar method can be used to calculate coupling constants for D2 Case.

TABLE IV. Convergence of ferroelectric polarization for D1-A structure along c-axis ($P_c$) calculated using GGA+U+vdW functional with respect to number of strings along z-direction in reciprocal space. The polarization quantum for the structure is 20.8622 $\mu\mathrm{C/cm}^2$.

| k-points | $P_c$ ($\mu\mathrm{C/cm}^2$) |
|---|---|
| $7 \times 7 \times 5$ | -10.16 |
| $7 \times 7 \times 10$ | -10.22 |
| $7 \times 7 \times 20$ | -10.17 |
| $10 \times 10 \times 15$ | -9.77 |
| $10 \times 10 \times 20$ | -9.75 |
| $10 \times 10 \times 25$ | -9.77 |

### Next-nearest-neighbour ($nnn$) Hamiltonian for D1 structure

In order to get the better estimation of $T_C$ for the D1-A structure, we have extracted the $nnn$ coupling constants by using the following extended Hamiltonian:

$$\begin{aligned} H = \sum_{i,j,k} J_{\parallel}^{I} \big[\vec{S}^{I,\alpha}_{i,j,k} \cdot \{\vec{S}^{I,\beta}_{i,j,k} + \vec{S}^{I,\beta}_{i-1,j,k} + \vec{S}^{I,\beta}_{i,j-1,k} + \vec{S}^{I,\beta}_{i-1,j-1,k}\}\big] \\ + J_{\parallel}^{II} [\vec{S}^{II,\alpha}_{i,j,k} \cdot \{\vec{S}^{II,\beta}_{i,j,k} + \vec{S}^{II,\beta}_{i-1,j,k} + \vec{S}^{II,\beta}_{i,j-1,k} + \vec{S}^{II,\beta}_{i-1,j-1,k}\}] \\ + J_{\perp} \sum_{i,j,k} \big[\vec{S}^{I,\alpha}_{i,j,k} \cdot \{\vec{S}^{II,\alpha}_{i,j,k-1} + \vec{S}^{II,\alpha}_{i,j,k+1}\} \\ + \vec{S}^{I,\beta}_{i,j,k} \cdot \{\vec{S}^{II,\beta}_{i,j,k-1} + \vec{S}^{II,\beta}_{i,j,k+1}\}\big] \\ + J_d \sum_{i,j,k} \big[\vec{S}^{I,\alpha}_{i,j,k} \cdot \{\vec{S}^{II,\beta}_{i,j,k} + \vec{S}^{II,\beta}_{i-1,j,k} + \vec{S}^{II,\beta}_{i,j,k-1} + \vec{S}^{II,\beta}_{i-1,j,k-1}\} \\ + \vec{S}^{II,\alpha}_{i,j,k} \cdot \{\vec{S}^{I,\beta}_{i,j,k} + \vec{S}^{I,\beta}_{i-1,j,k} + \vec{S}^{I,\beta}_{i,j,k+1} + \vec{S}^{I,\beta}_{i-1,j,k-1}\}\big] \end{aligned} \tag{15}$$

where $J_d$ is the $nnn$ coupling constants. Using Eq. 15, we extracted the $nnn$ coupling constant as given below

$$\boxed{J_d^{Cu-Mn} = \frac{E_F + E_G - E_C - E_A}{40}} \tag{16}$$

Using regular Metropolis Monte Carlo (MC) simulations[21], performing 100000 sweeps of the full simulation for thermalization and 50000 additional sweeps for equilibrium on a $8 \times 8 \times 8$ supercell, we sampled the configurations allowed by the above Hamiltonian . The temperature was varied in steps of 2 K around the magnetic ordering transition. We collected the average magnetic moments and the corresponding susceptibility at each temperature step.

### Monte-Carlo simulations of the as-calculated $nnn$ Heisenberg model

By using the extracted $nn$ and $nnn$ coupling constants, we performed Monte Carlo simulation and the Curie temperature was found to be 38K as illustrated in the Fig. 5 below.

## FERROELECTRIC POLARIZATION

Although our main aim was to tune the magnetic moment through mixed metal strategy in the parent polar Cu-MOF, we have also calculated the ferroelectric polarization through the Berry phase approach[12] using the GGA+$U$+vdW functional. We obtain the polarization as a difference between the polar ($\lambda = 1$) and non-polar ($\lambda = 0$) structures. Table IV shows the convergence of calculated $c$-axis polarization $P_c$ with respect to k-points mesh. Note that the polarization difference computed this way is one value in a lattice of values spaced by the polarization quantum. However, the actual value can be fixed by looking at the changes in the Berry phase along a smooth path connecting the polar and non-polar structures. The values reported in Table IV are chosen from such an analysis. Similarly, we also calculated the polarization along $c$-axis for the D0-G structure to be $-9.93\mu\mathrm{C/cm}^2$.

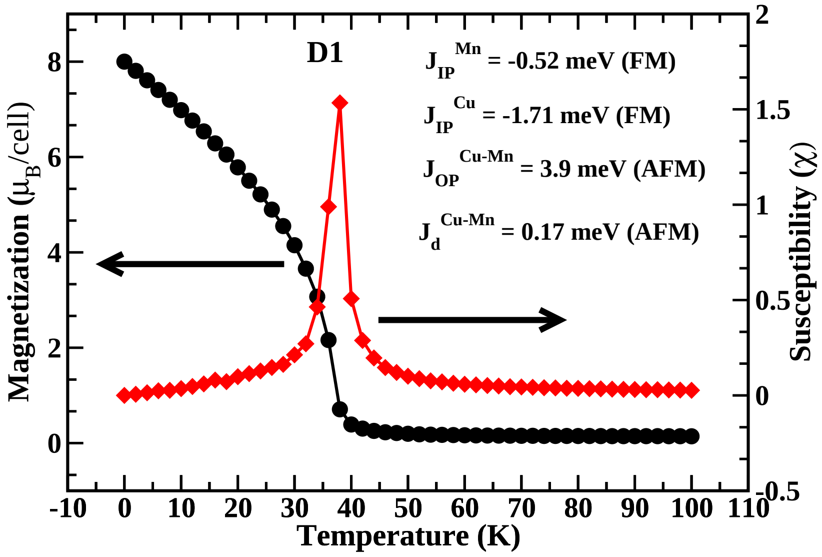


FIG. 5. Temperature-dependence of magnetic susceptibility and total magnetization obtained from classical Monte Carlo simulations for the D1-A structure using $nnn$ coupling constant (the ground-state)

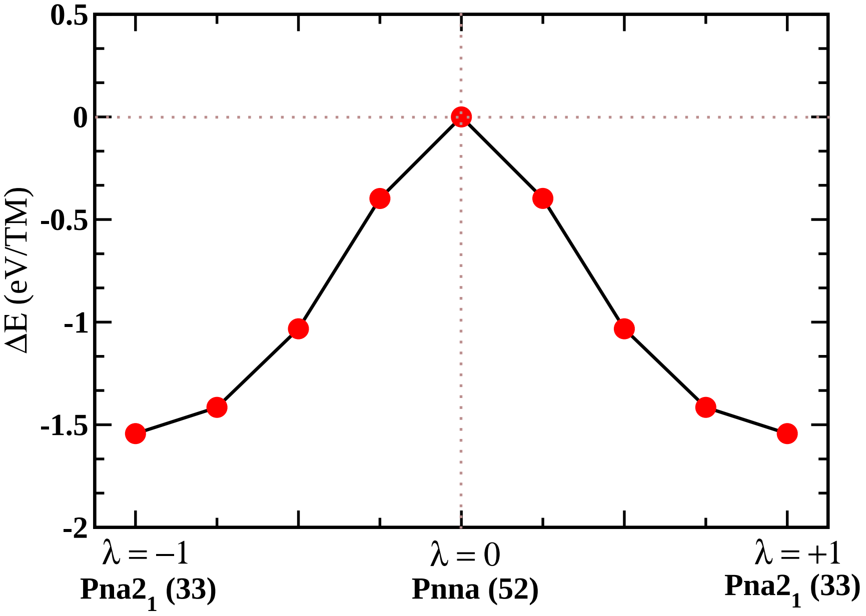


FIG. 6. The variation of total energy difference as a function of the structural distortion from paraelectric to the polar D0-G structure.

TABLE V. Total and partial polarization of A-site and $BX_3$ group for Cu-Mn MOF calculated from Berry phase approach. Polarization for the ideal structure is -8.01852 $\mu C/cm^2$ and the value of polarization quantum is 20.86218 $\mu C/cm^2$. $P_{polar}$ stands for the as calculated Berry phase value for polar structure. ΔP is the polarization difference between polar and ideal value.

| Structure | $P_{polar}$ ($\mu C/cm^2$) | ΔP ($\mu C/cm^2$) | Final polarization ($\mu C/cm^2$) (Quantum shift) |
|---|---|---|---|
| Polar | 3.0736 | 11.09212 | -9.77006 |
| A-site | 13.05467 | 21.07319 | 0.21101 **(Cu-MOF (≈ 0.21))** |
| $BX_3$ group | 5.48517 | 13.50369 | -7.35849 |
| B-site | -1.505 | 6.515 | 6.515 |
| X-site | 2.04264 | 10.06264 | -10.79954 |
| $A+BX_3$ | = 0.21101-7.35849= -7.14748 $\mu C/cm^2$ | | |
| $A+B+X_3$ | = 0.21101 +6.505- 10.80102= -4.08501 $\mu C/cm^2$ | | |

TABLE VI. Calculated dipole moments and the corresponding polarization by using localized basis code. The polarization was calculated for individual molecules of A-site cation and $BX_3$ group by considering the appropriate charge on each site and group.

| Structure | Dipole Moment (DM) (Debye) | | | Contribution from crystal positioning | | | Final DM (Debye) | Polarization $\mu C/cm^2$ |
|---|---|---|---|---|---|---|---|---|
| | Polar | Ideal | Total | Polar | Ideal | Total | | |
| **Cu-MOF** | | | | | | | | |
| A-site | 0.26 | 0.0 | 0.26 | 29.02 | 28.83 | 0.19 | 0.45 | 0.17 |
| $BX_3$ | -9.11 | -9.88 | 0.77 | 28.77 | 28.83 | -0.06 | 0.71 | 0.27 |
| $A+BX_3$ | | | | | | | 1.16 | 0.44 |
| **Cu-Mn-MOF** | | | | | | | | |
| A-site | 0.26 | 0.0 | 0.26 | 29.66 | 29.45 | 0.21 | 0.47 | 0.18 |
| $BX_3$ | -6.67 | 6.95 | -13.62 | 29.39 | 29.45 | -0.06 | -13.68 | -5.13 |
| $A+BX_3$ | | | | | | | -13.21 | -4.95 |

TABLE VII. Calculated magnetic moments ($\mu_B/cell$) for D1 structures at $\lambda = +1$.

| Total and atomic magnetic moments | $m_x$ | $m_y$ | $m_z$ |
|---|---|---|---|
| Total magnetic moments | -0.02 | 0.00 | -8.01 |
| Cu1 | -0.011 | -0.000 | 0.525 |
| Cu2 | -0.003 | 0.001 | 0.525 |
| Mn3 | 0.001 | 0.001 | -4.586 |
| Mn4 | 0.001 | -0.000 | -4.586 |

## MAGNETOELECTRIC EFFECT

In order to investigate the presence of magnetoelectric effect we carried out SOC calculations on the optimized D0-G and D1-A structures. In both cases we found small components of the magnetic moments in the $xy$-plane while the component along the $z$-axis remained as 4.0$\mu_B$ per TM ion. We also calculated the magnetic moments in the polarization inverted ($\lambda = -1$) structure and compared them with the $\lambda = +1$ case. The calculated values for the D1-A structure are reported in Tables VIII and VII, respectively. The data clearly shows that the magnetic moments in the $xy$-plane changes sign with inversion of the polarization confirming a magnetoelectric effect in the D1-A structure. Also given in the tables are the contributions to the moments from each TM ion in the supercell. The JT-active Cu ions are seen to be the major source for the off-axis moments. Since the number of these ions is lesser in the mixed metal MOF compared to the parent Cu-MOF the magnitude of the off-axis moments (0.01 $\mu_B$ per TM ion) are slightly lower than those in the parent MOF. Thus, the mixing in of non-JT ions leads to an apparent suppression of the magnetoelectric effect. Tables IX and X show the magnetic moments obtained for $\lambda = +1$ and $\lambda = -1$ structures of D0-G, respectively. In D0-G too the $xy$-plane magnetization alters direction with the inversion of the polarization indicating the presence of a magnetoelectric coupling.

## DENSITY OF STATES OF MIXED-METAL MOF

We have provided the electronic properties of the ground state magnetic MOF D1-A and the other feasible magnetic structure D0-G by plotting their corresponding density of states as shown in Figure 7 and 8, respectively. Fig. 7 (a) clearly shows that

TABLE VIII. Calculated magnetic moments ($\mu_B/cell$) for D1 structures at $\lambda = -1$.

| Total and atomic magnetic moments | $m_x$ | $m_y$ | $m_z$ |
|---|---|---|---|
| Total magnetic moments | 0.01 | 0.01 | -8.01 |
| Cu1 | 0.001 | 0.005 | 0.525 |
| Cu2 | 0.002 | -0.002 | 0.525 |
| Mn3 | 0.000 | 0.000 | -4.586 |
| Mn4 | 0.000 | 0.000 | -4.586 |

TABLE IX. Calculated magnetic moments ($\mu_B/cell$) for D0 structures at $\lambda = +1$.

| Total and atomic magnetic moments | $m_x$ | $m_y$ | $m_z$ |
|---|---|---|---|
| Total magnetic moments | -0.03 | -0.01 | -8.01 |
| Cu1 | -0.009 | -0.001 | 0.478 |
| Mn2 | -0.000 | -0.001 | -4.539 |
| Mn3 | 0.001 | 0.002 | -4.539 |
| Cu4 | -0.006 | -0.009 | 0.478 |

TABLE X. Calculated magnetic moments ($\mu_B/cell$) for D0 structures at $\lambda = -1$.

| Total and atomic magnetic moments | $m_x$ | $m_y$ | $m_z$ |
|---|---|---|---|
| Total magnetic moments | 0.00 | 0.01 | -8.01 |
| Cu1 | 0.000 | 0.004 | 0.476 |
| Mn2 | -0.001 | -0.002 | -4.536 |
| Mn3 | -0.000 | 0.001 | -4.536 |
| Cu4 | -0.001 | 0.000 | 0.476 |

the D1-A MOF is a ferrimagnetic insulator with a narrow band gap of 0.8 eV. The Mn majority ($3d$) states are fully occupied while the minority states are completely empty, which suggest that Mn exist in a $Mn^{2+}$ ($d^5$) high-spin valance state. The Cu d-projected DOS shows that most of the $d$ states are filled leaving a narrow empty band above the Fermi level with majority spin. This corresponds to the $e_g$ hole state and indicates that Cu is in the $Cu^{2+}$ ($d^9$) valence configuration. The DOS also reflects the AFM ordering in the structure. The valence configurations are also confirmed by the $d$-projected occupation numbers (not mentioned here). The DOS projected on oxygen states was also plotted in Fig. 7 (b) which indicates the strong overlapping of O $p$-orbitals with the occupied Mn $d$-orbitals. The DOS plotted in Figure 8 also shows that D0-G is also an insulator with band gap of 0.9 eV and has the same Mn and Cu valence configurations as D1-A.

## GGA RESULTS:

We have also investigated the structural, magnetic and electronic properties of our ($M_{0.5}M'_{0.5}$)-MOF by using just the GGA-PBE functional as it has been successfully used in the previous calculations[13]. We optimized all possible magnetic structures in D0, D1, D2 cation ordered environments. In this case, the ground state is the D0-G structure (Fig.9). We also extracted the coupling constants by using Eq. 3 and used those values to predict the transition temperature of the magnetic ground state by Monte Carlo simulations. The GGA predicted transition temperature is also much higher than the parent Cu-MOF as shown in Fig. 10. The DOS of the ground state D0-G structure indicates a vanishing band gap predicting the system to be metallic. To assess the importance of electron correlations in the $3d$ TM ions, we applied Hubbard U correction on top of GGA-optimized structures. Indeed, the correction opened up a gap in the D0 structure making the system insulating (see Fig. 11). As can be

TABLE XI. Comparison of energy differences $\Delta E$ (meV/cell) = $E_\gamma$ - $E_G$ (where $\gamma$ = A, C, G, FM) calculated using GGA, GGA+vdW, GGA+U, and GGA+U+vdW functionals for the GGA-optimized D0 structures.

| Magnetic ordering | GGA | GGA+vdW | GGA+U | GGA+U+vdW |
|---|---|---|---|---|
| A-type | 65 | 70 | 88 | 93 |
| C-type | 80 | 79 | 102 | 102 |
| G-type | 0 | 0 | 0 | 0 |
| FM | 141 | 145 | 197 | 202 |

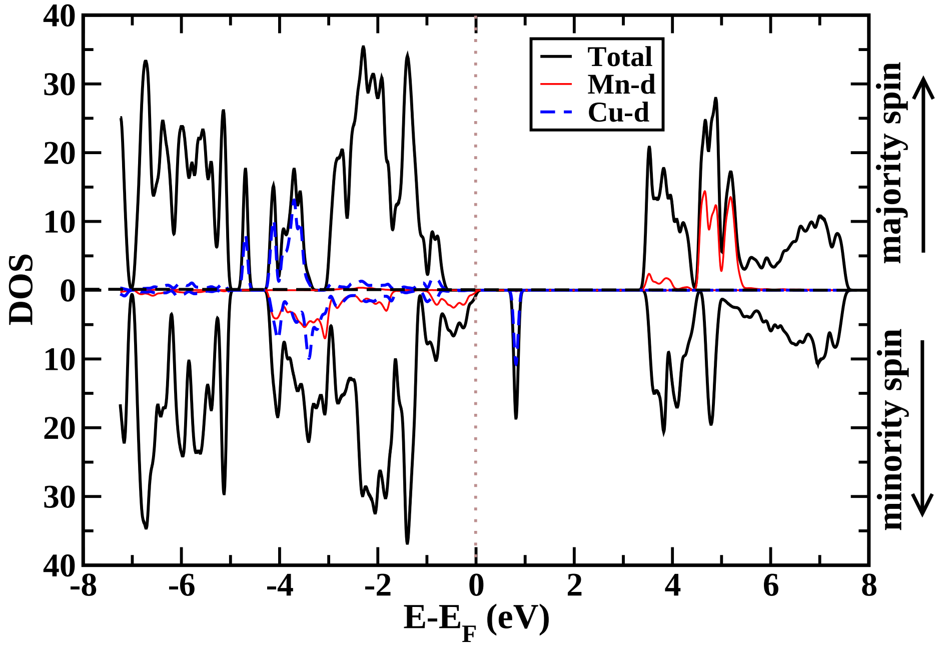


(a)

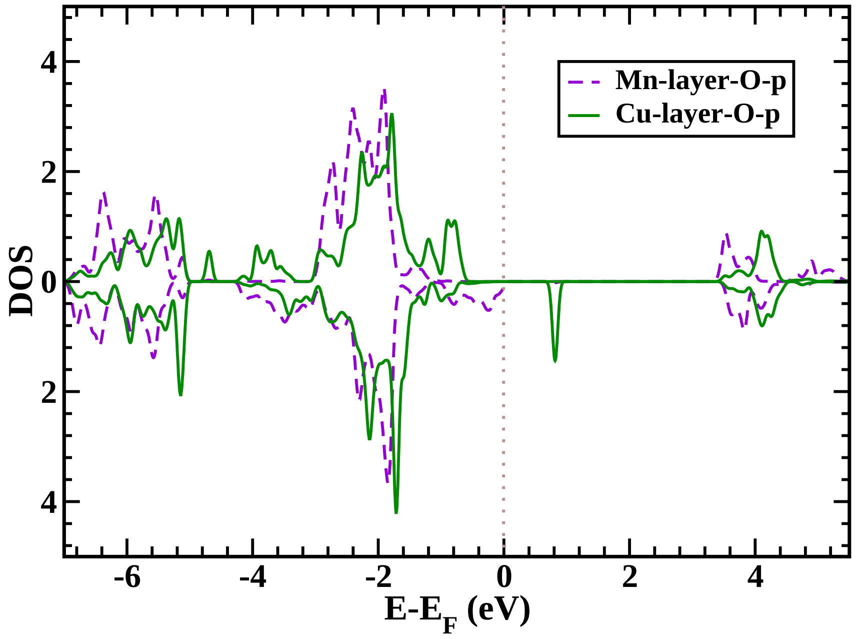


(b)

FIG. 7. Total and projected density of states in the D1-A structure in $Pna2_1$ phase: (a) Shows the GGA+U+vdW predicted density of states of total and projected DOS. Outer lines shows the total DOS and the inner solid lines indicates the total $d$-orbital contribution of Mn atoms and the dashed lines shows the $d$-orbital contribution of Cu atoms (b) Indicates the $p$-orbital contribution of O atoms connected to Mn and Cu layers.

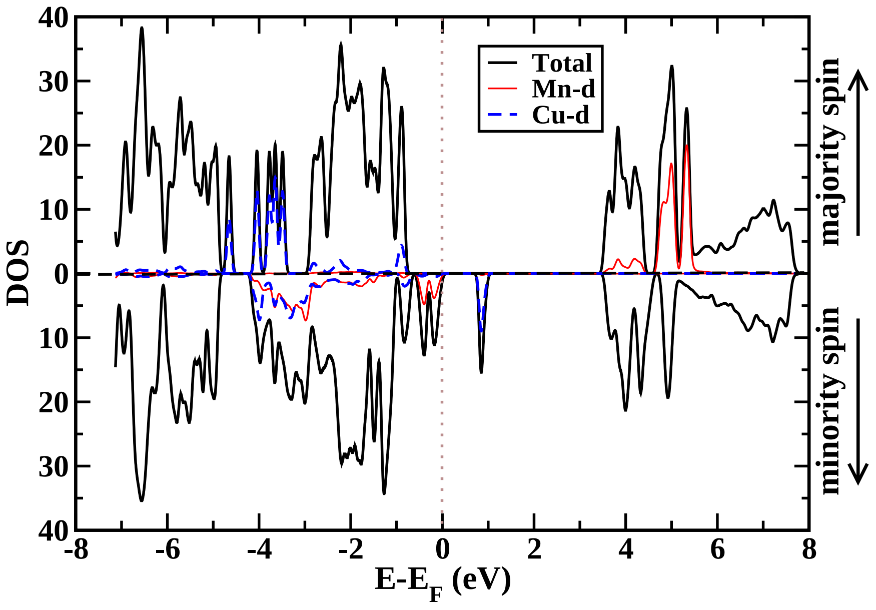


FIG. 8. Total and projected density of states in the polar D0-G structure.

seen in Table XI, the relative ordering of the various magnetic types is conserved and the relative energies only change slightly. However, adding U altered the ground sate from D0-G to D1-A, which is again a magnetic structure with a magnetic moment of $2\mu_B/TM$. The energies of various magnetic structures (A, C, G, FM) in D0, D1, D2 cation ordered states (relative to the corresponding D0-G energies) are listed in Tables XI, XII and XIII, respectively. The addition of a van der Waals correction serves to slightly increase (decrease) the relative energies of the D1 (D2) structures. Thus, it is primarily the electron correlations, through favorable magnetic exchange, which favor D1-A as the ground-state.

TABLE XII. Comparison of energy differences $\Delta E$ (meV/cell) = E$_\gamma$(D1) - E$_G$(D0) (where $\gamma$ = A, C, G, FM) calculated using GGA, GGA+vdW, GGA+U, and GGA+U+vdW functionals for the GGA-optimized D1 structures.

| Magnetic ordering | GGA | GGA+vdW | GGA+U | GGA+U+vdW |
|---|---|---|---|---|
| A-type | 78 | 85 | -256 | -249 |
| C-type | 185 | 193 | -136 | -128 |
| G-type | 99 | 107 | -218 | -210 |
| FM | 165 | 170 | -167 | -161 |

TABLE XIII. Comparison of energy differences $\Delta E$ (meV/cell) = E$_\gamma$(D2) - E$_G$(D0) (where $\gamma$ = A, C, G, FM) calculated using GGA, GGA+vdW GGA+U, and GGA+U+vdW functionals for the GGA-optimized D2 structures.

| Magnetic ordering | GGA | GGA+vdW | GGA+U | GGA+U+vdW |
|---|---|---|---|---|
| A-type | 171 | 168 | 158 | 155 |
| C-type | 55 | 46 | 45 | 37 |
| G-type | 104 | 97 | 87 | 80 |
| FM | 120 | 117 | 108 | 104 |

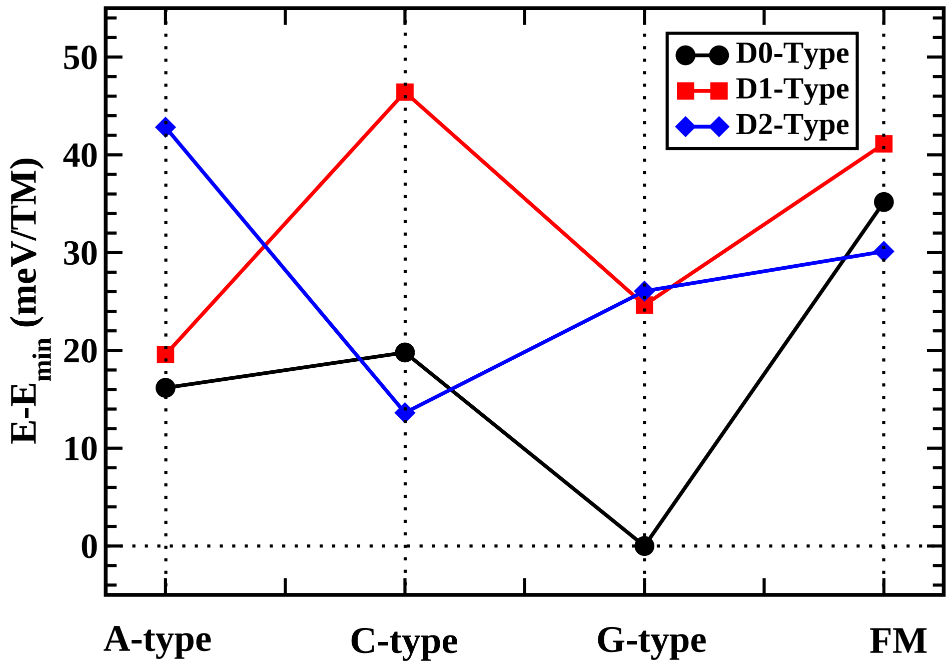


FIG. 9. Energies of GGA optimized various magnetic structures of D0, D1 and D2 cation ordering

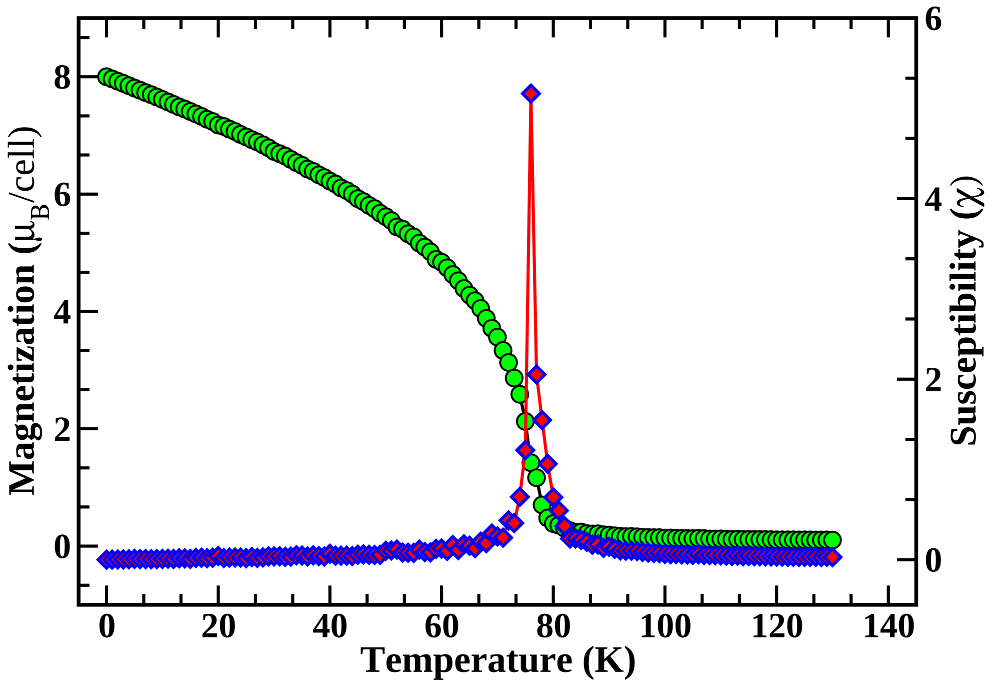


FIG. 10. The susceptibility and the total magnetization as a function of temperature from Monte-Carlo simulation. The susceptibility curve indicates that the ferrimagnetic curie temperature $(T_C)$ is 75 K. The total magnetization rapidly increases near $T_C$.

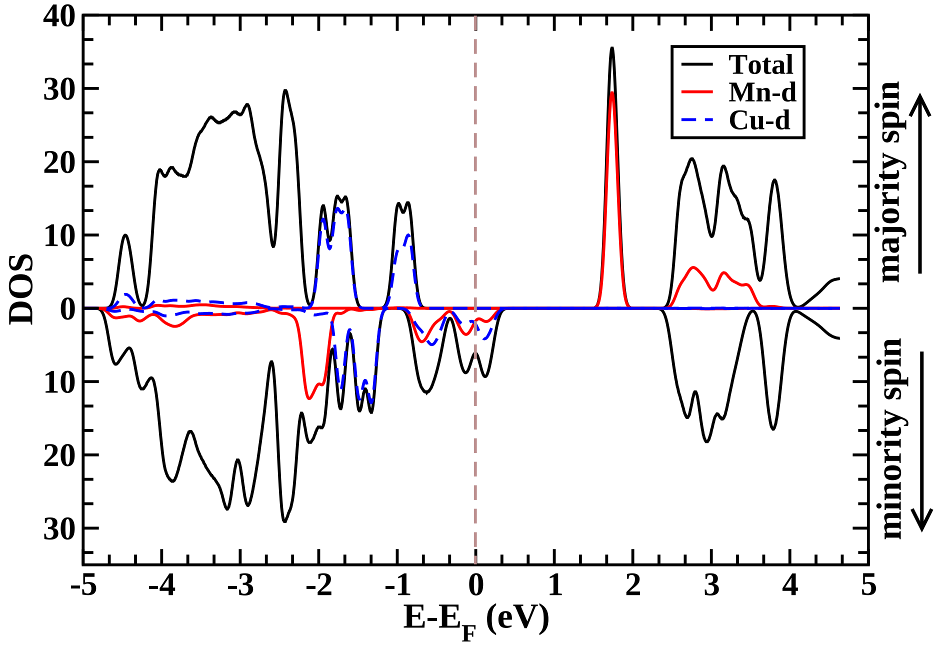


FIG. 11. Total and projected density of states of Cu-Mn-MOF (D0-G) structure in $Pna2_1$-like phase predicted using GGA functional.

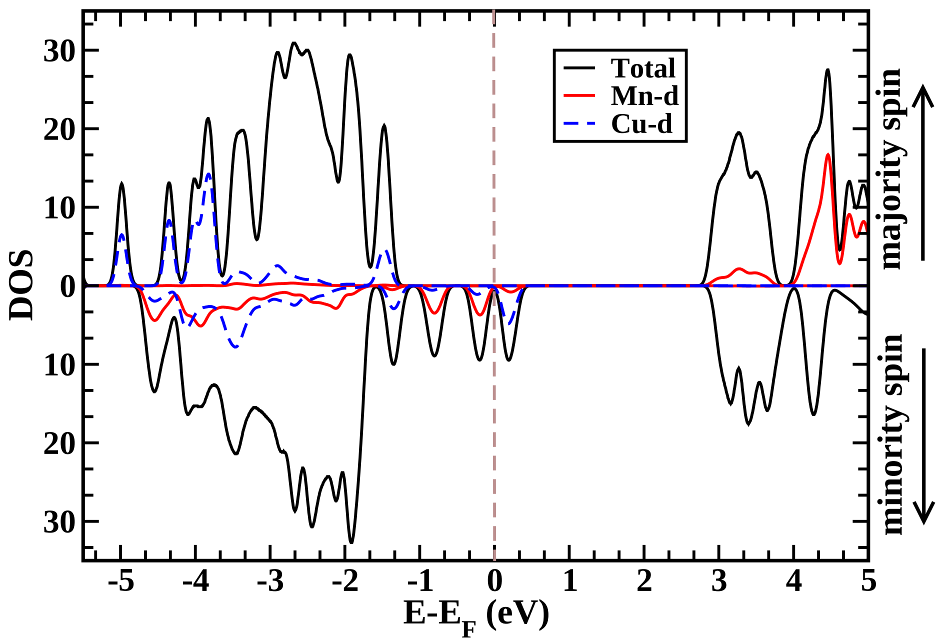


FIG. 12. Total and projected density of states of Cu-Mn-MOF (D0-G) structure in $Pna2_1$-like phase predicted using GGA+U functional on GGA-optimized structure.

[1] P. Giannozzi et al, J. Phys. Condens. Mater. **21**, 395502 (2006)
[2] J. P. Perdew, K. Burke, and M. Ernzerhof, Phys. Rev. Lett. **77**, 3865 (1996)
[3] J. P. Perdew, K. Burke, and M. Ernzerhof, Phys. Rev. Lett. **78**, 1396 (1997)
[4] P. E. Blöchl, Phys. Rev. B **50**, 17953 (1994)
[5] G. Kresse and D. Joubert, Phys. Rev. B **59**, 1758 (1999)
[6] V. I. Anisimov, F. Aryasetiawan, and A. I. Liechtenstein, J. Phys. Condens. Matter **9**, 767 (1997)
[7] H. J. Kulik and N. Marzari, J. Chem. Phys. **134**, 094103 (2011)
[8] H. J. Kulik and N. Marzari, J. Chem. Phys. **133**, 114103 (2010)
[9] M. Cococcioni and S. de Gironcoli, Phys. Rev. B **71**, 035105 (2005)
[10] B. Himmetoglu, R. M. Wentzcovitch, and M. Cococcioni, Phys. Rev. B **84**, 115108 (2011)
[11] H. J. Kulik, M. Cococcioni, D. A. Scherlis, and N. Marzari, Phys. Rev. Lett. **97**, 103001 (2006)
[12] R. D. King-Smith and D. Vanderbilt, Phys. Rev. B **47**, 1651 (1993)
[13] A. Stroppa, P. Jain, P. Barone, M. Marsman, J. M. Perez-Mato, A. K. Cheetham, H. W. Kroto, and S. Picozzi, Angew. Chem Int. Ed. **50**, 5847 (2011)
[14] Z. Xu, J. Rossmeisl, and J. R. Kitchin, J. Phys. Chem. C **119(9)**, 4827 (2015)
[15] A. Jain, G. Hautier, S. P. Ong, C. J. Moore, C. C. Fischer, K. A. Persson, and G. Ceder, Phys. Rev. B **84**, 045115 (2011)
[16] Z. Xu, Y. V. Joshi, S. Raman, and J. R. Kitchin, J. Chem. Phys. **142**, 144701 (2015)
[17] P. C. Rout, A. Putatunda, and V. Srinivasan, Phys. Rev. B **93**, 104415 (2016)
[18] S. Dengrong, S. Frangxiang, D. Xiaoyu, and L. Zhaohui, Inorg. Chem **54**, 8639 (2015)
[19] A. V. Krukau, O. A. Vydrov, A. F. Izmaylov, and G. E. Scuseria, J. Chem. Phys. **125**, 224106 (2006)
[20] K. L. Hu, M. Kurmoo, M. Wang, and S. Gao, Chem. Eur. J. **15**, 12050 (2009)
[21] R. F. L. Evans, W. J. Fan, P. Chureemart, T. A. Ostler, M. O. A. Ellis, and R. W. Chantrell, J. Phys. Condens. Matter **26**, 103202 (2014)
[22] E. Kroumova, M. I. Aroyo, J. M. Perez-Mato, S. Ivantchev, J. M. Igartua, and H. Wondratschek, J. Appl. Crystallogr. **34**, 783 (2001)
[23] D. Orobengoa, C. Capillas, M. I. Aroyo, and J. M. Perez-Mato, J. Appl. Crystallogr. **42**, 840 (2009)
